# Supplementary material for: A Density-Based Basis-Set Correction For Wave Function Theory
Source: arXiv:1904.10913 source file (2019-05-16)
Supplement: Supplementary file 1 [file G2_srDFT-SI.pdf]

# Supplementary Information for “A Density-Based Basis-Set Correction For Wave Function Theory”

Pierre-François Loos,<sup>1, a)</sup> Bathélemy Pradines,<sup>2, 3</sup> Anthony Scemama,<sup>1</sup> Julien Toulouse,<sup>2, b)</sup> and Emmanuel Giner<sup>2, c)</sup>

<sup>1)</sup>Laboratoire de Chimie et Physique Quantiques (UMR 5626), Université de Toulouse, CNRS, UPS, France

<sup>2)</sup>Laboratoire de Chimie Théorique, Sorbonne Université, CNRS, Paris, France

<sup>3)</sup>Institut des Sciences du Calcul et des Données, Sorbonne Université, Paris, France

## I. LOCAL-DENSITY APPROXIMATION

The local-density approximation (LDA) of the ECMD complementary functional is defined as

$$\bar{E}_{\text{LDA}}^B[n, \mu^B] = \int n(\mathbf{r}) \bar{\epsilon}_{\text{c,md}}^{\text{sr,LDA}}(n(\mathbf{r}), \zeta(\mathbf{r}), \mu^B(\mathbf{r})) d\mathbf{r}, \quad (1)$$

where  $\zeta = (n_{\uparrow} - n_{\downarrow})/n$  is the spin polarization and  $\bar{\epsilon}_{\text{c,md}}^{\text{sr,LDA}}(n, \zeta, \mu)$  is the ECMD short-range correlation energy per electron of the uniform electron gas (UEG)<sup>1</sup> parameterized in Ref. 2. The short-range LDA correlation functional relies on the transferability of the physics of the UEG which is certainly valid for large  $\mu$  but is known to over correlate for small  $\mu$ .

The sensitivity with respect to the RS-DFT functional is quite large for the double- and triple- $\zeta$  basis sets, where clearly the PBE functional performs better. However, from the quadruple- $\zeta$  basis, the LDA and PBE functionals agree within a few tenths of a kcal/mol. Such weak sensitivity to the density-functional approximation when reaching large basis sets shows the robustness of the approach.

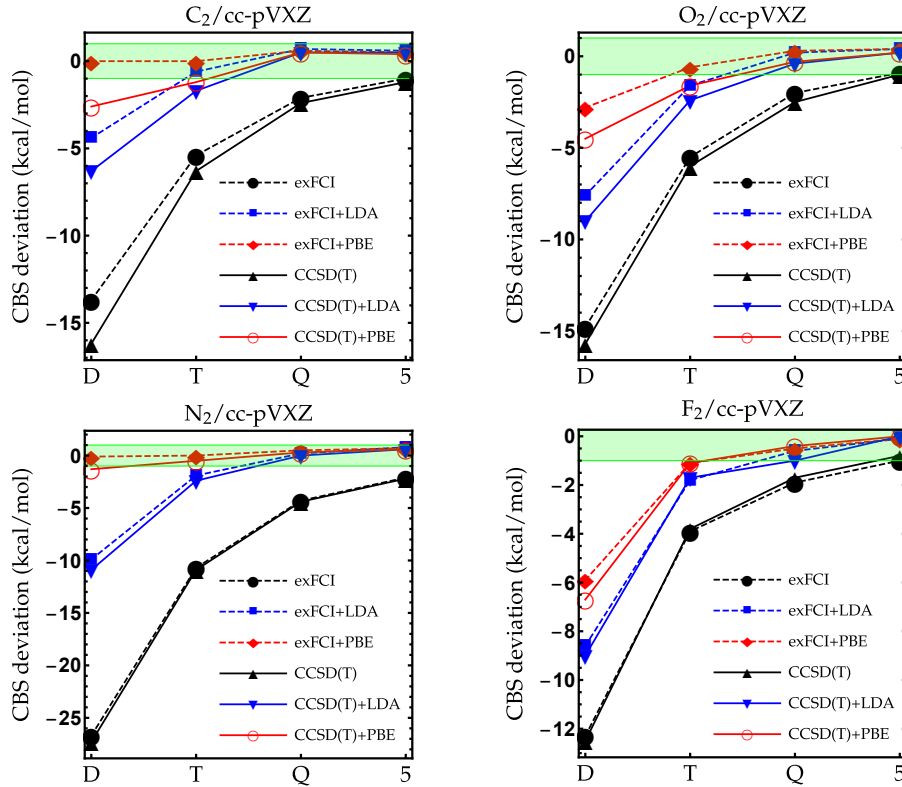

FIG. 1. Deviation (in kcal/mol) from CBS atomization energies of C<sub>2</sub> (top left), O<sub>2</sub> (top right), N<sub>2</sub> (bottom left) and F<sub>2</sub> (bottom right) obtained with various methods and basis sets. The green region corresponds to chemical accuracy (i.e. error below 1 kcal/mol).

<sup>a)</sup>Electronic mail: [loos@irsamc.ups-tlse.fr](mailto:loos@irsamc.ups-tlse.fr)

<sup>b)</sup>Electronic mail: [toulouse@lct.jussieu.fr](mailto:toulouse@lct.jussieu.fr)

<sup>c)</sup>Electronic mail: [emmanuel.giner@lct.jussieu.fr](mailto:emmanuel.giner@lct.jussieu.fr)



TABLE II. Frozen-core atomization energies (in kcal/mol) of  $C_2$ ,  $O_2$ ,  $N_2$  and  $F_2$  computed with various methods and basis sets. The deviations with respect to the corresponding CBS values are reported in parenthesis. See main text for more details.

| Molecule | Method      | Dunning's basis set cc-pVXZ |              |             |             | CBS   |
|----------|-------------|-----------------------------|--------------|-------------|-------------|-------|
|          |             | X = D                       | X = T        | X = Q       | X = 5       |       |
| $C_2$    | exFCI       | 132.0(−13.7)                | 140.3(−5.4)  | 143.6(−2.1) | 144.7(−1.0) | 145.7 |
|          | exFCI+LDA   | 141.3(−4.4)                 | 145.1(−0.6)  | 146.4(+0.7) | 146.3(+0.6) |       |
|          | exFCI+PBE   | 145.7(+0.0)                 | 145.7(+0.0)  | 146.3(+0.6) | 146.2(+0.5) |       |
|          | CCSD(T)     | 129.2(−16.2)                | 139.1(−6.3)  | 143.0(−2.4) | 144.2(−1.2) | 145.4 |
|          | CCSD(T)+LDA | 139.1(−6.3)                 | 143.7(−1.7)  | 145.9(+0.5) | 145.9(+0.5) |       |
|          | CCSD(T)+PBE | 142.8(−2.6)                 | 144.2(−1.2)  | 145.9(+0.5) | 145.8(+0.4) |       |
| $N_2$    | exFCI       | 201.1(−26.7)                | 217.1(−10.7) | 223.5(−4.3) | 225.7(−2.1) | 227.8 |
|          | exFCI+LDA   | 217.9(−9.9)                 | 225.9(−1.9)  | 228.0(+0.2) | 228.6(+0.8) |       |
|          | exFCI+PBE   | 227.7(−0.1)                 | 227.8(+0.0)  | 228.3(+0.5) | 228.5(+0.7) |       |
|          | CCSD(T)     | 199.9(−27.3)                | 216.3(−10.9) | 222.8(−4.4) | 225.0(−2.2) | 227.2 |
|          | CCSD(T)+LDA | 216.3(−10.9)                | 224.8(−2.4)  | 227.2(−0.0) | 227.8(+0.6) |       |
|          | CCSD(T)+PBE | 225.9(−1.3)                 | 226.7(−0.5)  | 227.5(+0.3) | 227.8(+0.6) |       |
| $O_2$    | exFCI       | 105.2(−14.8)                | 114.5(−5.5)  | 118.0(−2.0) | 119.1(−0.9) | 120.0 |
|          | exFCI+LDA   | 112.4(−7.6)                 | 118.4(−1.6)  | 120.2(+0.2) | 120.4(+0.4) |       |
|          | exFCI+PBE   | 117.2(−2.8)                 | 119.4(−0.6)  | 120.3(+0.3) | 120.4(+0.4) |       |
|          | CCSD(T)     | 103.9(−16.1)                | 113.6(−6.0)  | 117.1(−2.5) | 118.6(−1.0) | 119.6 |
|          | CCSD(T)+LDA | 110.6(−9.0)                 | 117.2(−2.4)  | 119.2(−0.4) | 119.8(+0.2) |       |
|          | CCSD(T)+PBE | 115.1(−4.5)                 | 118.0(−1.6)  | 119.3(−0.3) | 119.8(+0.2) |       |
| $F_2$    | exFCI       | 26.7(−12.3)                 | 35.1(−3.9)   | 37.1(−1.9)  | 38.0(−1.0)  | 39.0  |
|          | exFCI+LDA   | 30.4(−8.6)                  | 37.2(−1.8)   | 38.4(−0.6)  | 38.9(−0.1)  |       |
|          | exFCI+PBE   | 33.1(−5.9)                  | 37.9(−1.1)   | 38.5(−0.5)  | 38.9(−0.1)  |       |
|          | CCSD(T)     | 25.7(−12.5)                 | 34.4(−3.8)   | 36.5(−1.7)  | 37.4(−0.8)  | 38.2  |
|          | CCSD(T)+LDA | 29.2(−9.0)                  | 36.5(−1.7)   | 37.2(−1.0)  | 38.2(+0.0)  |       |
|          | CCSD(T)+PBE | 31.5(−6.7)                  | 37.1(−1.1)   | 37.8(−0.4)  | 38.2(+0.0)  |       |

TABLE III. Deviation from the reference CCSD(T)/CBS atomization energies (in kcal/mol) for various methods and basis sets. See main text for more details.

| Molecule                                     | CCSD(T)/CBS | Deviation from CBS atomization energies |         |         |         |         |             |         |         |         |                        |
|----------------------------------------------|-------------|-----------------------------------------|---------|---------|---------|---------|-------------|---------|---------|---------|------------------------|
|                                              |             | CCSD(T)                                 |         |         |         |         | CCSD(T)+LDA |         |         |         |                        |
|                                              |             | cc-pVDZ                                 | cc-pVTZ | cc-pVQZ | cc-pV5Z | cc-pV7Z | cc-pVDZ     | cc-pVTZ | cc-pVQZ | cc-pV7Z | CCSD(T)+PBE<br>cc-pVTZ |
| BeH                                          | 50.12       | -3.38                                   | -1.01   | -0.36   | -0.19   | -0.75   | -0.75       | -0.03   | 0.04    | -0.75   | -0.03                  |
| C <sub>2</sub> H <sub>2</sub>                | 403.00      | -22.99                                  | -8.69   | -3.43   | -1.76   | -5.12   | -5.12       | -1.08   | 0.37    | -5.12   | -1.08                  |
| C <sub>2</sub> H <sub>4</sub>                | 561.69      | -27.16                                  | -9.44   | -3.59   | -1.84   | -4.88   | -4.88       | -0.56   | 0.58    | -4.88   | -0.56                  |
| C <sub>2</sub> H <sub>6</sub>                | 710.81      | -32.62                                  | -10.65  | -3.97   | -2.03   | -5.28   | -5.28       | -0.20   | 0.76    | -5.28   | -0.20                  |
| CH                                           | 83.89       | -5.96                                   | -1.97   | -0.75   | -0.39   | -0.81   | -0.81       | -0.03   | 0.15    | -0.81   | -0.03                  |
| CH <sub>2</sub> <sup>1</sup> A <sub>1</sub>  | 180.61      | -10.99                                  | -3.57   | -1.34   | -0.68   | -1.55   | -1.55       | 0.00    | 0.29    | -1.55   | 0.00                   |
| CH <sub>2</sub> <sup>3</sup> B <sub>1</sub>  | 189.94      | -8.82                                   | -2.78   | -1.0    | -0.51   | -1.87   | -1.87       | -0.38   | 0.00    | -1.87   | -0.38                  |
| CH <sub>3</sub>                              | 306.81      | -14.33                                  | -4.47   | -1.62   | -0.83   | -2.33   | -2.33       | -0.08   | 0.27    | -2.33   | -0.08                  |
| CH <sub>3</sub> Cl                           | 395.02      | -20.77                                  | -8.34   | -3.35   | -1.72   | -4.38   | -4.38       | -0.16   | -0.16   | -4.38   | -0.16                  |
| CH <sub>4</sub>                              | 419.19      | -18.35                                  | -5.64   | -2.01   | -1.03   | -2.55   | -2.55       | 0.18    | 0.51    | -2.55   | 0.18                   |
| CN                                           | 179.32      | -14.98                                  | -7.26   | -3.18   | -1.63   | -2.16   | -2.16       | -0.82   | 0.20    | -2.16   | -0.82                  |
| CO                                           | 258.64      | -11.01                                  | -5.94   | -2.60   | -1.33   | -0.93   | -0.93       | 0.44    | 0.44    | -0.93   | 0.44                   |
| CO <sub>2</sub>                              | 388.29      | -20.79                                  | -10.95  | -4.67   | -2.39   | -3.19   | -3.19       | -1.69   | 0.60    | -3.19   | -1.69                  |
| CS                                           | 170.82      | -10.72                                  | -6.25   | -2.88   | -1.47   | -1.94   | -1.94       | -1.58   | -0.16   | -1.94   | -1.58                  |
| Cl <sub>2</sub>                              | 59.33       | -8.26                                   | -5.23   | -2.49   | -1.28   | -3.63   | -3.63       | -2.46   | -0.90   | -3.63   | -2.46                  |
| ClF                                          | 62.43       | -8.51                                   | -4.83   | -2.33   | -1.19   | -4.02   | -4.02       | -2.23   | -0.81   | -4.02   | -2.23                  |
| ClO                                          | 64.35       | -11.86                                  | -6.35   | -3.16   | -1.62   | -5.99   | -5.99       | -3.08   | -1.25   | -5.99   | -3.08                  |
| F <sub>2</sub>                               | 38.24       | -6.62                                   | -3.52   | -1.72   | -0.88   | -3.17   | -3.17       | -1.54   | -0.48   | -3.17   | -1.54                  |
| H <sub>2</sub> CO                            | 373.18      | -19.31                                  | -8.07   | -3.31   | -1.70   | -2.84   | -2.84       | -0.70   | 0.50    | -2.84   | -0.70                  |
| H <sub>2</sub> O                             | 222.78      | -15.21                                  | -8.83   | -2.37   | -1.21   | -4.03   | -4.03       | -1.07   | -0.14   | -4.03   | -1.07                  |
| H <sub>2</sub> O <sub>2</sub>                | 268.77      | -22.78                                  | -9.44   | -4.08   | -2.09   | -6.64   | -6.64       | -2.06   | -0.30   | -6.64   | -2.06                  |
| H <sub>2</sub> S                             | 183.36      | -10.66                                  | -4.33   | -1.55   | -0.79   | -2.50   | -2.50       | -1.16   | -0.12   | -2.50   | -1.16                  |
| H <sub>3</sub> COH                           | 512.25      | -28.32                                  | -10.40  | -4.10   | -2.10   | -5.95   | -5.95       | -1.17   | 0.31    | -5.95   | -1.17                  |
| H <sub>3</sub> CSH                           | 473.92      | -25.84                                  | -10.02  | -3.88   | -1.98   | -5.49   | -5.49       | -1.79   | -0.01   | -5.49   | -1.79                  |
| HCN                                          | 311.54      | -20.86                                  | -9.06   | -3.80   | -1.95   | -3.59   | -3.59       | -0.85   | -0.37   | -3.59   | -0.85                  |
| HCO                                          | 277.92      | -15.04                                  | -6.87   | -2.84   | -1.46   | -2.38   | -2.38       | -0.89   | 0.37    | -2.38   | -0.89                  |
| HCl                                          | 107.31      | -5.64                                   | -2.46   | -0.93   | -0.48   | -1.37   | -1.37       | -0.81   | -0.22   | -1.37   | -0.81                  |
| HF                                           | 141.67      | -8.45                                   | -3.48   | -1.42   | -0.73   | -2.70   | -2.70       | -0.96   | -0.23   | -2.70   | -0.96                  |
| HOCl                                         | 165.85      | -15.82                                  | -7.34   | -3.28   | -1.68   | -5.39   | -5.39       | -2.29   | -0.62   | -5.39   | -2.29                  |
| Li <sub>2</sub>                              | 24.10       | -0.78                                   | -0.30   | -0.07   | -0.04   | 0.39    | 0.39        | 0.13    | 0.1     | 0.39    | 0.13                   |
| LiF                                          | 138.33      | -10.78                                  | -4.56   | -1.95   | -1.0    | -3.30   | -3.30       | -0.91   | -0.30   | -3.30   | -0.91                  |
| LiH                                          | 57.70       | -4.15                                   | -1.05   | -0.38   | -0.20   | -0.71   | -0.71       | 0.12    | 0.11    | -0.71   | 0.12                   |
| N <sub>2</sub>                               | 227.18      | -18.66                                  | -9.41   | -4.20   | -2.15   | -2.26   | -2.26       | -0.90   | 0.20    | -2.26   | -0.90                  |
| N <sub>2</sub> H <sub>4</sub>                | 437.39      | -36.95                                  | -14.25  | -5.83   | -2.99   | -8.13   | -8.13       | -1.60   | -0.01   | -8.13   | -1.60                  |
| NH                                           | 82.86       | -8.10                                   | -3.02   | -1.24   | -0.63   | -1.51   | -1.51       | -0.22   | -0.06   | -1.51   | -0.22                  |
| NH <sub>2</sub>                              | 182.14      | -15.31                                  | -5.61   | -2.26   | -1.16   | -3.16   | -3.16       | -0.50   | -0.03   | -3.16   | -0.50                  |
| NH <sub>3</sub>                              | 297.46      | -21.21                                  | -7.62   | -3.01   | -1.54   | -4.42   | -4.42       | -0.62   | 0.07    | -4.42   | -0.62                  |
| NO                                           | 151.73      | -13.87                                  | -7.26   | -3.25   | -1.66   | -2.20   | -2.20       | -1.10   | 0.08    | -2.20   | -1.10                  |
| Na <sub>2</sub>                              | 16.44       | -0.71                                   | -0.14   | -0.06   | -0.03   | 0.20    | 0.20        | 0.15    | 0.08    | 0.20    | 0.15                   |
| NaCl                                         | 99.61       | -11.48                                  | -5.41   | -2.26   | -1.16   | -4.34   | -4.34       | -2.13   | -0.52   | -4.34   | -2.13                  |
| O <sub>2</sub>                               | 119.64      | -9.86                                   | -5.34   | -2.40   | -1.23   | -3.08   | -3.08       | -1.72   | -0.30   | -3.08   | -1.72                  |
| OH                                           | 107.08      | -8.37                                   | -3.27   | -1.34   | -0.69   | -2.23   | -2.23       | -0.63   | -0.08   | -2.23   | -0.63                  |
| P <sub>2</sub>                               | 115.68      | -18.05                                  | -9.34   | -4.00   | -2.05   | -3.96   | -3.96       | -1.89   | 0.26    | -3.96   | -1.89                  |
| PH <sub>2</sub>                              | 153.91      | -11.50                                  | -4.32   | -1.51   | -0.77   | -2.56   | -2.56       | -0.82   | 0.16    | -2.56   | -0.82                  |
| PH <sub>3</sub>                              | 241.49      | -15.43                                  | -5.80   | -2.03   | -1.04   | -3.12   | -3.12       | -1.03   | 0.20    | -3.12   | -1.03                  |
| S <sub>2</sub>                               | 103.07      | -12.76                                  | -7.34   | -3.28   | -1.68   | -5.69   | -5.69       | -3.18   | -0.95   | -5.69   | -3.18                  |
| SO                                           | 125.12      | -10.77                                  | -6.14   | -2.94   | -1.51   | -3.33   | -3.33       | -2.10   | -0.59   | -3.33   | -2.10                  |
| SO <sub>2</sub>                              | 258.09      | -22.35                                  | -13.90  | -6.75   | -3.46   | -5.16   | -5.16       | -4.67   | -1.32   | -5.16   | -4.67                  |
| Si <sub>2</sub>                              | 75.74       | -10.01                                  | -4.47   | -1.82   | -0.93   | -4.19   | -4.19       | -1.49   | 0.30    | -4.19   | -1.49                  |
| Si <sub>2</sub> H <sub>6</sub>               | 535.58      | -27.32                                  | -10.13  | -3.46   | -1.77   | -5.59   | -5.59       | -1.86   | 0.30    | -5.59   | -1.86                  |
| SiH <sub>2</sub> <sup>1</sup> A <sub>1</sub> | 153.66      | -8.72                                   | -2.98   | -0.98   | -0.50   | -3.51   | -3.51       | -1.46   | -0.34   | -3.51   | -1.46                  |
| SiH <sub>2</sub> <sup>3</sup> B <sub>1</sub> | 133.17      | -6.68                                   | -2.40   | -0.73   | -0.37   | -3.02   | -3.02       | -1.57   | -0.49   | -3.02   | -1.57                  |
| SiH <sub>3</sub>                             | 227.99      | -10.53                                  | -3.72   | -1.15   | -0.59   | -1.82   | -1.82       | -0.74   | 0.12    | -1.82   | -0.74                  |
| SiH <sub>4</sub>                             | 324.59      | -14.10                                  | -4.88   | -1.52   | -0.78   | -1.91   | -1.91       | -0.58   | 0.33    | -1.91   | -0.58                  |
| SiO                                          | 191.48      | -11.34                                  | -6.72   | -3.15   | -1.61   | -0.76   | -0.76       | -1.18   | 0.12    | -0.76   | -1.18                  |
